# Supplementary material for: Empowering Retrieval-based Conversational Recommendation with Contrasting User Preferences
Source: arXiv:2503.22005 source file (2025-03-27)
Supplement: Supplementary file 1 [file appendix.tex]

%%
%% If your work has an appendix, this is the place to put it.
\appendix
