# Supplementary material for: Empowering Retrieval-based Conversational Recommendation with Contrasting User Preferences
Source: arXiv:2503.22005 source file (2025-03-27)
Supplement: Supplementary file 2 [file tab_appendix_null_augmentaion.tex]

% Please add the following required packages to your document preamble:
% \usepackage{booktabs}
% \usepackage{multirow}
% \usepackage{graphicx}
\begin{table}[]\scriptsize
\centering
\resizebox{\textwidth}{!}{%
\begin{tabular}{@{}cc|c|cc|cc@{}}
\toprule
\multicolumn{2}{c|}{\multirow{2}{*}{Dataset}} & \multirow{2}{*}{\#samples} & \multicolumn{2}{c|}{Extraction}    & \multicolumn{2}{c}{Augmentation}   \\ \cmidrule(l){4-7} 
\multicolumn{2}{c|}{}                         &                            & \#null of like & \#null of dislike & \#null of like & \#null of dislike \\ \midrule
\multicolumn{1}{c|}{\multirow{3}{*}{\spearl}}    & Train & 45,913 & 53  & 8,878  & 0 & 4      \\
\multicolumn{1}{c|}{}                          & Valid & 4,978  & 0   & 935    & 0 & 0      \\
\multicolumn{1}{c|}{}                          & Test  & 2,268  & 1   & 425    & 0 & 1      \\ \midrule
\multicolumn{1}{c|}{\multirow{3}{*}{\sinspired}} & Train & 1,634  & 45  & 897    & 0 & 5      \\
\multicolumn{1}{c|}{}                          & Valid & 193    & 4   & 132    & 0 & 0      \\
\multicolumn{1}{c|}{}                          & Test  & 196    & 9   & 110    & 0 & 0      \\ \midrule
\multicolumn{1}{c|}{\multirow{3}{*}{\sredial}}   & Train & 20,579 & 411 & 16,766 & 3 & 16,210 \\
\multicolumn{1}{c|}{}                          & Valid & 2,278  & 52  & 1,882  & 0 & 1,818  \\
\multicolumn{1}{c|}{}                          & Test  & 2,686  & 121 & 2,305  & 2 & 2,181  \\ \bottomrule
\end{tabular}%
}
\caption{}
\label{tab:appendix_null_augmentation}
\end{table}
